# Supplementary material for: LifeBench: A Benchmark for Long-Horizon Multi-Source Memory
Source: arXiv:2603.03781 source file (2026-03-04)
Supplement: Supplementary file 1 [file appendix.tex]

\section{Data Structure}
\label{sec:data-structure}
\begin{itemize}
    \item \textbf{Topic Events}: topic events are major events within one year. Topic events belong to \todo{xxx} types of events including ``Career and Education'', ``Relationships'', ``Living Situation'', ``Social and Life Style'', ``Finance'', ``Entertainment'', ``Personal Grow'', ``Unexpected Events'', ``Health and Well-being'', ``Other''. Example: ``Neck Rehabilitation Training Program'' belongs to ``Health and Well-being''. 
    \item \textbf{Stage Events}: A stage event is a mid-level event structure characterized by temporal continuity and semantic coherence. It can be aggregated upward into thematic events and decomposed downward into atomic events. A stage event typically consists of a sequence of observable actions that occur continuously over a period of time and revolve around a single, unified objective.
    \item \textbf{Atomic Events}: atomic events have a duration of less than one day. Atomic events are generated by decomposing topic events. Example: for the event ``Neck Rehabitation Training'' can be decomposed into atomic events such as ``discussion of the neck rehabilitation'', etc. Atomic Events have the same schema with topic event except that atomic events are sub-events of topic events.
    % \item \textbf{Mid-term Event}: mid-term events are similar to atomic events, except that mid-term events last for several days or weeks.
    \item \textbf{User Profile}: list the important properties
    \item \textbf{Daily Event}: Some Daily events can be generated from atomic events, while some daily events are not generated from atomic events. \todo{Add an examples}.

    \item \textbf{Phone Operations}
\end{itemize}

\begin{table*}[!htbp]
    \centering
    \resizebox{\textwidth}{!}{
    \begin{tabular}{l|l|l}
        \toprule
        \multicolumn{3}{c}{Topic Events} \\
        \midrule    
        EventId & Formatted Numbers& Numbered of the form parentid \\
        Name & Text & Description of the topic events\\
        Type & Category & \makecell[l]{``Career and Education'', ``Relationships'', ``Living Situation'',\\ ``Social and Life Style'', ``Finance'', ``Entertainment'', ``Personal Grow'',\\ ``Unexpected Events'', ``Health and Well-being'', ``Other''}\\
        Date & Time & The start and end time of the topic event\\
        Description & Text & The description of whole process of the topic event\\
        Participant & Name and Relation & The person involved in the event and the relation with the main role\\
        Location & Text & The location of the event\\
        SubEvent & Structure & The subevent of the topic event with the same structure\\ 
        \toprule
    \end{tabular}
    }
    \caption{Properties of the topic events}
    \label{tab:placeholder}
\end{table*}

\section{Simulated Generation Process}

Event Inference Module: generate topic events, decompose topic events to mid-term events or atomic events. The maximum number of layers is 3. 


\begin{enumerate}
    \item \textbf{Topic Event Generation} \\
    Given profile, generate topic events. In other words, we need to model $P(topic\_event|profile)$
    
     To improve authenticity, we model $p(topic\_event|topic\_event\_type)$ and $p(topic\_event\_type|profile)$. We control probability of $p(topic\_event\_type|profile)$, whereas $p(topic\_event|topic\_event\_type)$ is from LLM. \todo{How to get more diverse profile and topic event types?} Specifically:
    \begin{enumerate}
        \item First, we classify topic events: by clustering 40,000 topic events generated from 100 profiles, we identify $X$ topic event categories.
        \item Then, we construct a ``profile-topic event category'' dataset and train an MLP model to model the probability of a profile generating a specific topic event category. \todo{refer to the concept of ``topic event distribution''. The number of topic event types?}
    \end{enumerate}

    \item \textbf{Event Graph Expansion} \\
    \todo{clarify how the topic events are generated from topic event distribution} We sample 300 topic events for each individual based on topic event generation model p(topic event| topic event distribution). Subsequently, the sampled topic events are planned and decomposed. Each topic event can be decomposed into 3 levels of event hierarchy. A topic event can be connected to a mid-level event, which is then decomposed into atomic events.

    Event decomposition is implemented via a large language model (LLM) that analyzes the duration and importance of each topic event for hierarchical decomposition $P(event|parent\_event, profile)$. 

    \begin{algorithm}[h]
        \caption{Atomic Event Extraction via DFS and LLM Decomposition}
        \label{alg:atomic_event_extraction}
        \begin{algorithmic}[1]
            % Clear input/output (single-line to avoid numbering errors)
            \Require{EventTree $T$ (rooted tree; nodes = events, leaves = candidate events); LLM with two functions: isAtomic(e) (returns True if e is atomic, else False) and decomposeEvent(e) (returns list of finer-grained sub-events of e)}
            \Ensure{Updated EventTree $T$ (all leaves are atomic events); List of all atomic events $\mathcal{A}$}
            
            \State $\mathcal{A} \gets \emptyset$ % Initialize atomic event list
            
            % Recursive DFS function (no \ForEach)
            \Function{DFS-Process}{$node$}
                \If{$node$ is a leaf node of $T$}
                    % Check atomicity with LLM
                    \State $is\_atomic \gets \text{isAtomic}(\text{event of } node)$
                    \If{$is\_atomic$}
                        \State $\mathcal{A} \gets \mathcal{A} \cup \{\text{event of } node\}$
                        \Return
                    \Else
                        % Decompose non-atomic event into sub-events
                        \State $sub\_events \gets \text{decomposeEvent}(\text{event of } node)$
                        \State $n \gets \text{length of } sub\_events$ % Get number of sub-events
                        
                        % Replace \ForEach with index-based \For loop
                        \For{$i \gets 1$ \textbf{to} $n$}
                            \State $sub\_e \gets sub\_events[i]$ % Get i-th sub-event (1-indexed)
                            \State Create new child node $child$ with event = $sub\_e$
                            \State Add $child$ as a child of $node$ in $T$ (node becomes internal)
                        \EndFor
                        
                        % Process child nodes with index-based \For loop
                        \State $m \gets \text{number of children of } node$
                        \For{$j \gets 1$ \textbf{to} $m$}
                            \State $child \gets \text{j-th child of } node$
                            \State \Call{DFS-Process}{$child$}
                        \EndFor
                    \EndIf
                \Else
                    % Process children of internal nodes (index-based \For)
                    \State $m \gets \text{number of children of } node$
                    \For{$j \gets 1$ \textbf{to} $m$}
                        \State $child \gets \text{j-th child of } node$
                        \State \Call{DFS-Process}{$child$}
                    \EndFor
                \EndIf
            \EndFunction
            
            % Start DFS from the tree root
            \State \Call{DFS-Process}{$\text{root of } T$}
            
            \Return $T, \mathcal{A}$
        \end{algorithmic}
    \end{algorithm}

    
    \todo{has been done ,see the algorithm 1.[add more details of the procedure-- change this into a graph expansion procedure, i.e. select a leaf then generate its subevent]}. This process ultimately yields atomic events corresponding to each topic event.

    The generation and decomposition of each topic event can be done in parallel. Our assumption is that mid-events and atomic events depend only on its parent topic event. 

    \item \textbf{Daily Activity Simulation} \\
    Schedule atomic events and and generate daily events. We generate use $P(daily\_event_{ij}|atomic\_event_i, profile, memory)$ where $i$ indicates the $i-th$ day and $j$ indicates the daily event $j$ of the $i$ day. We use  LLM for the whole process.
    We organize the atomic events into a schedule format and design human-like agents to simulate an individual's daily life, thereby generating their daily activities. The specific simulation process includes:
    \begin{itemize}
        \item Subjective thinking and planning
        \item Objective logic adjustment
        \item Integration of real POI (Point of Interest) data
        \item Event enrichment and reflection
        \item Memory and cognition updates
    \end{itemize}

    This process is most time-consuming. We consider the speculative decoding.

    \item \textbf{Generating Mobile Phone Operations} \\
    \todo{Use LLm for synthetizing phone operation given daily events p(po|daily event). Change the following process to modeling ``daily events as hidden variables'', which can be inferred from log data (profile, phone operations) using expectation maximization process (think of K-means algorithm where cluster id are hidden). We can pretrain the models of P(po|daily event) and p(daily event|profile, topic event distribution) from synthetic data. The process of discovering hidden variables (daily events and then atomic events) can be moved to KG construction.}
    We aim to model the conditional probability of mobile operations given daily events, user profiles, and inherent noise:
\[
p(\mathcal{O} \mid \mathcal{E}, \mathcal{P}, \mathcal{N})
\]
where:
- $\mathcal{O}$ = mobile operations (APP usage, calls, SMS, push notifications),
- $\mathcal{E}$ = predefined daily event types (to protect privacy and ensure inference accuracy),
- $\mathcal{P}$ = user profiles (age, occupation, usage preferences),
- $\mathcal{N}$ = intrinsic noise (random ads, public welfare/weather alerts, service reminders).

Using real-world mobile operation and user profile datasets, we propose a two-stage framework: first infer predefined daily event types from $\mathcal{O}$ and $\mathcal{P}$ (avoiding sensitive details), then train a diffusion model to generate realistic $\mathcal{O}$ conditioned on $\mathcal{E}$, $\mathcal{P}$, and $\mathcal{N}$. The workflow is as follows:

\begin{itemize}
    \item \textbf{Construct Dataset} \\
    Pair mobile operations with corresponding daily event types via the information of profile and phone data. Aligned samples are defined as:
    \[
    \mathcal{D}_{\text{align}} = \{ (\mathcal{E}_i, \mathcal{P}_j, \mathcal{O}_k, \mathcal{N}_m) \mid \mathcal{O}_k, \mathcal{P}_j  \}
    \]

    \item \textbf{Mobile Operation Embedding} \\
    Convert discrete operation data into low-dimensional latent vectors:
    Discrete types (Operation name): Word2Vec embedding: $\mathbf{e}_{\mathcal{O}}^{\text{disc}} = \text{Word2Vec}(\mathcal{O}.\text{type})$
    Text types (SMS content): LLM-based semantic embedding: $\mathbf{e}_{\mathcal{O}}^{\text{text}} = \text{LLMEmbed}(\mathcal{O}.\text{content})$
    Numerical types (duration): Normalization: $\mathbf{e}_{\mathcal{O}}^{\text{num}} = \text{Normalize}(\mathcal{O}.\text{value})$
    Final embedding:
    \[
    \mathbf{e}_{\mathcal{O}} = \text{Concatenate}(\mathbf{e}_{\mathcal{O}}^{\text{disc}}, \mathbf{e}_{\mathcal{O}}^{\text{text}}, \mathbf{e}_{\mathcal{O}}^{\text{num}})
    \]

    \item \textbf{Daily Event and Profile Encoding} \\
    Encode conditional variables into unified guidance vectors:
    Fusion with noise:
    \[
    \mathbf{e}_{\text{cond}} = \text{Concatenate}(\mathbf{e}_{\mathcal{E}}, \mathbf{e}_{\mathcal{P}}, \mathbf{e}_{\mathcal{N}})
    \]
    where $\mathbf{e}_{\mathcal{N}} \sim \mathcal{N}(0, \sigma^2 I)$ is noise embedding.

    \item \textbf{Diffusion Model Training} \\
    Train a conditional diffusion model to learn $\mathcal{O}$ distribution:
    - Forward process (noise addition):
    \[
    \mathbf{e}_{\mathcal{O}}^t = \sqrt{\bar{\alpha}_t} \mathbf{e}_{\mathcal{O}}^0 + \sqrt{1-\bar{\alpha}_t} \epsilon
    \]
    where $\bar{\alpha}_t = \prod_{s=1}^t \alpha_s$, $\alpha_s=1-\beta_s$, $\epsilon \sim \mathcal{N}(0,I)$.
    
    - Reverse process (denoising): Train $\epsilon_\theta$ to predict noise:
    \[
    \mathcal{L} = \mathbb{E} \left\| \epsilon - \epsilon_\theta(\mathbf{e}_{\mathcal{O}}^t, \mathbf{e}_{\text{cond}}, t) \right\|_2^2
    \]

    \item \textbf{Generation Inference} \\
    Generate operations from random noise via iterative denoising:
    1. Initialize: $\mathbf{e}_{\mathcal{O}}^T \sim \mathcal{N}(0,I)$
    2. Denoise for $t=T$ to $1$:
    \[
    \mathbf{e}_{\mathcal{O}}^{t-1} = \frac{1}{\sqrt{\alpha_t}} \left( \mathbf{e}_{\mathcal{O}}^t - \frac{\beta_t}{\sqrt{1-\bar{\alpha}_t}} \epsilon_\theta \right) + \sqrt{\beta_t} z
    \]
    3. Map to discrete operations via cosine similarity:
    \[
        \hat{\mathcal{O}} = \arg\max_{\mathcal{O}} \text{cosine}(\hat{\mathbf{e}}_{\mathcal{O}}^0, \mathbf{e}_{\mathcal{O}}^0)
    \]
\end{itemize}
    \todo{revise the generation process}.
    % After obtaining an individual's daily events, we generate potential mobile phone operations based on their daily life. Specifically:
    % \begin{enumerate}
    %     \item We train a ``atomic event-mobile phone operation'' probability model using real-world data.
    %     \item Based on this probability model, corresponding mobile phone operations are generated from the atomic events.
    % \end{enumerate}
\end{enumerate}

\section{Evaluate}
It can be divided into three parts: profile clustering, data extraction, and analysis and verification. 

\textbf{Similar Profile, Similar Phone Operation}: Based on this assumption, we designed a method to verify whether the synthetic data's persona and mobile phone behavior conform to real-world situations. We match the relatively realistic data with the persona, and then use the KNN algorithm to find the K most realistic persona profiles that are closest to the synthetic data's persona. Based on our assumption, the mobile phone behavior of the synthetic data should have similarity to the mobile phone behavior of these K people. Then, we calculate the JS divergence to judge whether the synthetic data conforms to real-world scenarios.

\textbf{Location, Mobile Factuality Metric}: Here, we use a large model to extract location data, and then use Amap (Gaode Maps) tools to verify the authenticity of the locations and the reasonableness of the travel time. Travel times that do not match Amap's predicted travel time are considered unreasonable.

\textbf{Event Faithfulness}: 1) recall non-existing events; 2) planing but not following events. To do that we need: First, we use a large model to extract events and the dates that the corresponding events should occur according to their descriptions. Then, we compare each event with all the behaviors within that date and use the large model to determine whether these behaviors actually occurred. However, considering that the actual event dates may vary slightly due to various reasons, we give the dates a buffer period that extends forward or backward; events occurring within this buffer period are considered reasonable.

\textbf{Unexpected person}: We use a language model to extract the characters who appear in the event, and then search in the character profile to determine whether the appearance of the character in the plot is reasonable or whether a character that should not appear in the plot has appeared.

\section{Knowledge Graph Construction Process}
\todo{1) Noise vs daily event driven phone operation classification; 2) Estimate Topic Event distribution based on profile and long-term phone operations (consider using noise/not-noise phones -- some advertising is driven by real-world operations); 3) Daily event inference: daily events are considered as hidden variables, and we aim to infer daily events given phone operations, profile, and (possibly) the inferred topic event distribution.}

\begin{enumerate}

\item \textbf{Atomic Event Extraction}
We parse JSON-formatted mobile phone data (including calls, SMS, push notifications, calendar entries, and notes). For each data record, we extract structured atomic events that contain type, participants, location, description, and timestamp. The description is generated by combining the original phone data with semantic understanding from a LLM. Atomic events represent the most granular level of mobile phone activities.

\item \textbf{Entity Alignment and Fusion}

\paragraph{Cross-Source Person Entity Alignment}
We integrate person-related information from multiple data sources, including contact names, call records, SMS participants, and calendar attendees. These discrete data points are merged into unified Person nodes through entity matching and alias recognition, eliminating redundancy, and ensuring consistency of person entities across the knowledge graph.

\paragraph{Location Fusion and Normalization}
We collect location information from multiple sources, including GPS coordinates, points of interest (POI), and location-related text from SMS and calendar entries. Through systematic normalization and disambiguation, these multi-source location data are converted into unified Location nodes, ensuring standardized spatial representation in the knowledge graph.

\item \textbf{Multi-Layer Event Clustering and Thematic Event Recognition}
\todo{can simplify this process into estimating topic event distribution from a sequence of phone operations and profile}

\paragraph{middle-Level Event Clustering}
We group atomic events by date and perform clustering within each day . Clustering is based on time windows and semantic similarity. Each cluster represents a potential middle topic event. We extract key attributes that include the name, type, temporal range, participants, and locations of the event. These middle topic events form the intermediate layer of the hierarchical event structure.

\paragraph{top-Level Event Clustering}
We also aggregate middle topic events by week to generate top topic events. Top clustering considers semantic relatedness, shared participants, and common locations. The resulting top topic events represent higher-level patterns and longer-duration activities. This multi-layer approach ensures manageable input sizes for LLM processing while maintaining semantic coherence.

\item \textbf{Hierarchical Knowledge Graph Construction}

We construct a multi-layer knowledge graph consisting of three event levels: atomic events (bottom layer), middle thematic events (intermediate layer), and top topic events (top layer). Hierarchical relationships are explicitly encoded, where each higher-level event contains references to its constituent lower-level events. Additionally, we incorporate unified Person and Location entities, creating cross-modal connections between persons, locations, and events at each hierarchical level.

\item \textbf{Knowledge Graph Output and Management}

The final knowledge graph is serialized as a JSON structure containing:
\begin{itemize}
    \item \texttt{atomic\_events}: atomic-level events with complete metadata
    \item \texttt{middle\_topic\_events}: aggregated events at the middle-level
    \item \texttt{weekly\_topic\_events}: aggregated events at the top-level
    \item \texttt{unified\_persons}:  standardized person entities with alias mappings
    \item \texttt{unified\_locations}:  standardized location entities with type classifications
    \item \texttt{metadata}: Comprehensive statistics and temporal coverage information
\end{itemize}

\end{enumerate}
